# Supplementary material for: Visualising Geographically-Embedded Origin-Destination Flows: in 2D and immersive environments
Source: arXiv:1908.00662 source file (2019-08-06)
Supplement: Supplementary file 1 [file chapter-appendix.tex]

\chapter{Appendix}
\label{sec:appendix}
